# Supplementary material for: A metalanguage for cost-aware denotational semantics
Source: arXiv:2209.12669 source file (2022-09-26)
Supplement: Supplementary file 1 [file appendix-calfiter.tex]

\section{Model for \calfiter{}}
